# Supplementary material for: Occupational Disorder as the Origin of Flattening of the Acoustic Phonon Branches in the Clathrate Ba$_{8}$Ga$_{16}$Ge$_{30}$
Source: arXiv:2301.08371 ancillary file (2023-01-20)
Supplement: Supplementary file 1 [file SI_thermoelectric.pdf]

# Supplementary Information for "Occupational Disorder as the Origin of Flattening of Phonon Branches in the Clathrate $Ba_8Ga_{16}Ge_{30}$"

Susmita Roy,[1] Tyler C. Sterling,[1] Dan Parshall,[1,2] Eric S. Toberer,[3]
Mogens Christensen,[4] Devashibhai T. Adroja,[5] and Dmitry Reznik[1,6,*]

[1]*Department of Physics, University of Colorado at Boulder, Boulder, Colorado 80309, USA*
[2]*Department of Economics, Universidad del Rosario, Calle 12C 6-25, Bogota, 111711, D.C., Colombia*
[3]*Department of Physics, Colorado School of Mines, Golden, Colorado 80401, USA*
[4]*Department of Chemistry and Interdisciplinary Nanoscience Center (iNANO), Aarhus University Langelandsgade 140, Aarhus, 8000, Denmark*
[5]*ISIS Facility, STFC, Rutherford Appleton Laboratory, Chilton, Oxfordshire OX11 0QX, United Kingdom Funding*
[6]*Center for Experiments on Quantum Materials, University of Colorado at Boulder, Boulder, Colorado 80309, USA*

(Dated: November 17, 2022)

## I. COMPARISON TO PREVIOUSLY PUBLISHED RESULTS

In the main text, we present time-of-flight (TOF) inelastic-neutron-scattering (INS) data taken recently and compare our measurements to DFT calculations. Here, we compare our calculations to the results by Christensen et al. where the large-gap avoided crossing due to the rattler atom was observed [1].

The neutron scattering spectra S($\mathbf{Q}$,$\omega$) calculated from the ordered and disordered unit cells both satisfactorily reproduce the intensities in the zones where the avoided crossings in the branches along [h,h,0] were measured (figure 1) [1]. However, the ordered cell calculation produces a few notable differences from experiment. There are flat optical modes at ∼4 meV and ∼6 meV that are not present in the experimental data. In the disordered cell calculation, the intensity in these regions is much weaker and broader.

We can also compare our calculations to Raman spectroscopy. In ref. [2], Raman spectra of $X_8Ga_{16}Ge_{30}$ with X∈ {Ba, Eu, Sr} are measured and effects of "off centering" are observed for the X=Eu and X=Sr compounds. There is no offcentering in the Ba compound, consistent with our results. We only discuss the X=Ba Raman data here. Ref. [2] does not investigate disorder, but it is fruitful to compare our calculations to their Raman spectra and look for effects of disorder here. Calculating Raman intensities from DFT is outside the scope of this paper, so we cannot compare directly to their measurements; rather, we choose to calculate $S(\boldsymbol{Q},\omega)$ with $\boldsymbol{Q} = (3,3,0)$ to compare to Raman scattering. At this zone center ($\boldsymbol{q} = 0$), the acoustic phonons are weak and the low energy optical phonons are strong. We broaden the spectrum with a Gaussian with FWHM=0.5 meV to approximate the energy resolution in Raman scattering.

At first glance the neutron spectra in fig. 2a) don't resemble the Raman intensity; the neutron intensity is dominated by phonons with $E \gtrsim 75.$ cm$^{-1}$. However, the peak energies and linewidths are similar. We can improve the analysis by comparing calculations from the ordered vs. disordered crystal and by "switching off" scattering from different atoms in the neutron calculation. In fig. 2b) we set the Ba neutron scattering lengths to 0 ($b_{Ba} = 0$); the scattering in this panel is entirely from the Ga and Ge atoms. Conversely in fig. 2c) we set the scattering from Ga and Ge to 0 ($b_{Ga} = b_{Ge} = 0$); here, the scattering is entirely from the Ba atoms. Note the y-axis in c) is different than a) and b): there are fewer Ba atoms in

* dmitry.reznik@colorado.edu

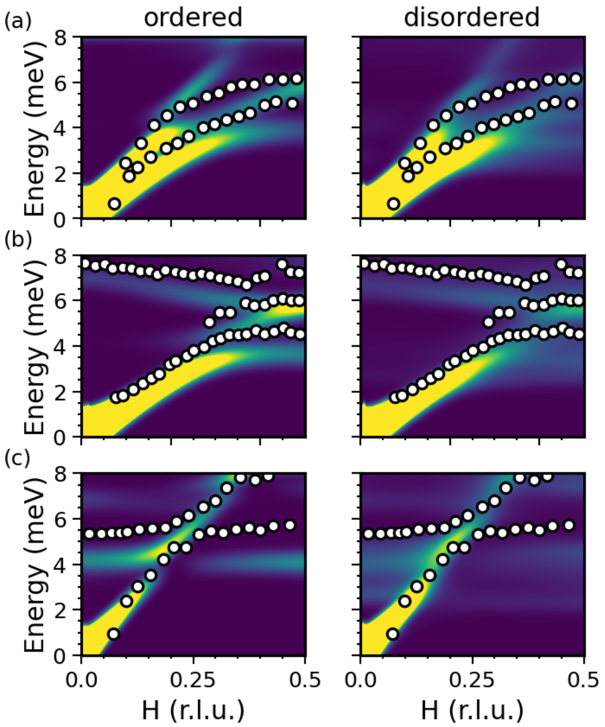


FIG. 1. Inelastic neutron scattering structure factors S($\mathbf{Q}$,$\omega$) calculated from the ordered $Ba_8Ga_{16}Ge_{30}$ unit cell are shown in the left column and from the disordered $Ba_8Ga_{16}Ge_{30}$ unit cell are in the right column. (a) Theoretical S($\mathbf{Q}$,$\omega$) along $\mathbf{Q}$=(2+h,2+h,2). (b) Theoretical S($\mathbf{Q}$,$\omega$) along $\mathbf{Q}$=(h,h,4). (c) Theoretical S($\mathbf{Q}$,$\omega$) along $\mathbf{Q}$=(3+h,3+h,0). The structure factors in the disordered phase are averaged over all equivalent directions assuming cubic symmetry. The circles in all panels are experimental data from ref. [1].

the crystal than Ga/Ge, so the intensity is lower for Ba phonons.

The Ba peak positions and widths in fig. 2c) from the disordered calculation agree well with the Raman peaks identified as Ba phonons in ref. [2]. Moreover, the optical phonons with $E \gtrsim 75$ cm$^{-1}$ agree well the Ga/Ge peaks in b). Somewhat lower energies in the calculation compared with experiment are due to use of GGA in the DFT calculation: GGA is known to predict bonds that are softer than they actually are.

It is clear that the disordered calculation matches lineshapes of the Raman peaks much better than the ordered calculation does. Thus, we conclude that the Raman spectra support our claims that disorder causes splitting of the Ba phonons in $Ba_8Ga_{16}Ge_{30}$ resulting in broad Ba optical phonon peaks.

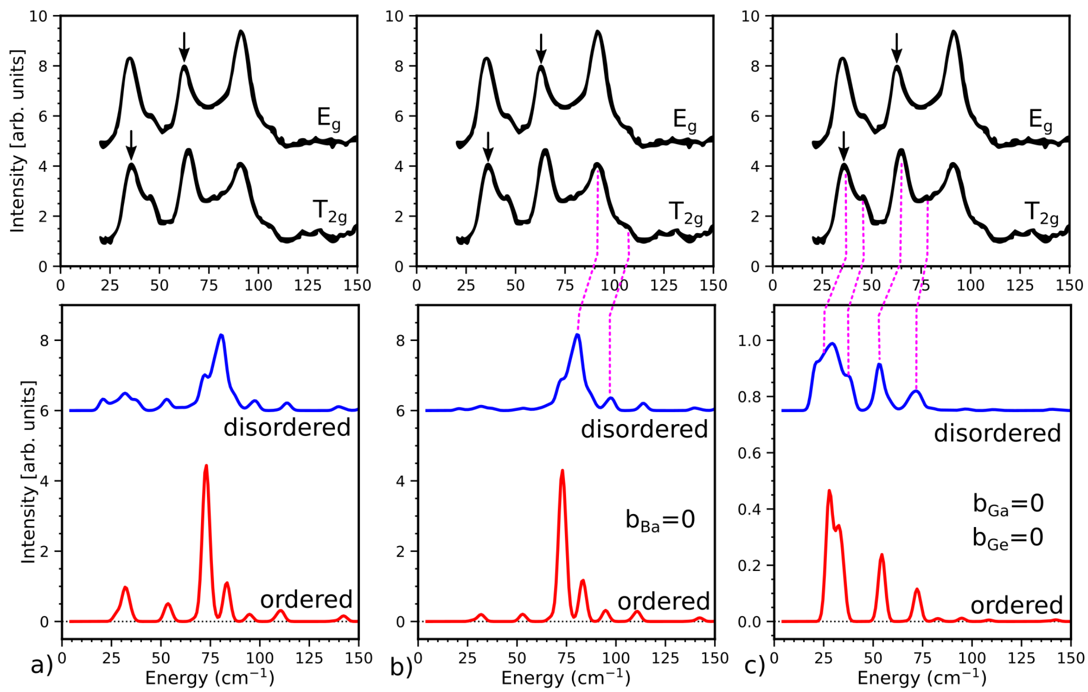


FIG. 2. Comparison of calculated inelastic neutron scattering intensity at a zone center $\boldsymbol{Q} = (3, 3, 0)$ to experimental Raman scattering spectra of Ref. [[2]] a) $S(\boldsymbol{Q}, \omega)$ with all scattering lengths set to their physical values, b) with Ba scattering lengths set to 0, and c) with Ga and Ge scattering lengths set to 0. All panels in the top row are the same and are repeated for clarity: the two curves are experimental Raman spectra with different polarizations and Ba optical phonon peaks labeled by their symmetry: the arrow labels the Ba phonons . The neutron spectra are broadened using a Gaussian with FWHM=0.5 meV. The correspondence between Ba phonons and Ga/Ge phonons and the peaks in the Raman spectra is obvious from panels b) and c): dashed lines are a guide to the eye. Only peak positions and widths should be compared. Raman and neutron intensities from peak to peak are expected to be different due to different coupling mechanisms.

## II. APPROXIMATE RESOLUTION FUNCTION

We compared generalized (i.e. neutron-weighted) densities of states (GDoS) measured at two different incident energies ($E_i = 22$ meV and $E_i = 52$ meV) to our calculations in the main text. Our goal here was a *quantitative* comparison, so it was essential to broaden our calculated $\mathrm{S}(\mathbf{Q}, \omega)$ with an accurate approximation of the experimental energy resolution. We determined the resolution by looking at incoherent $E = 0$ intensity away from Bragg

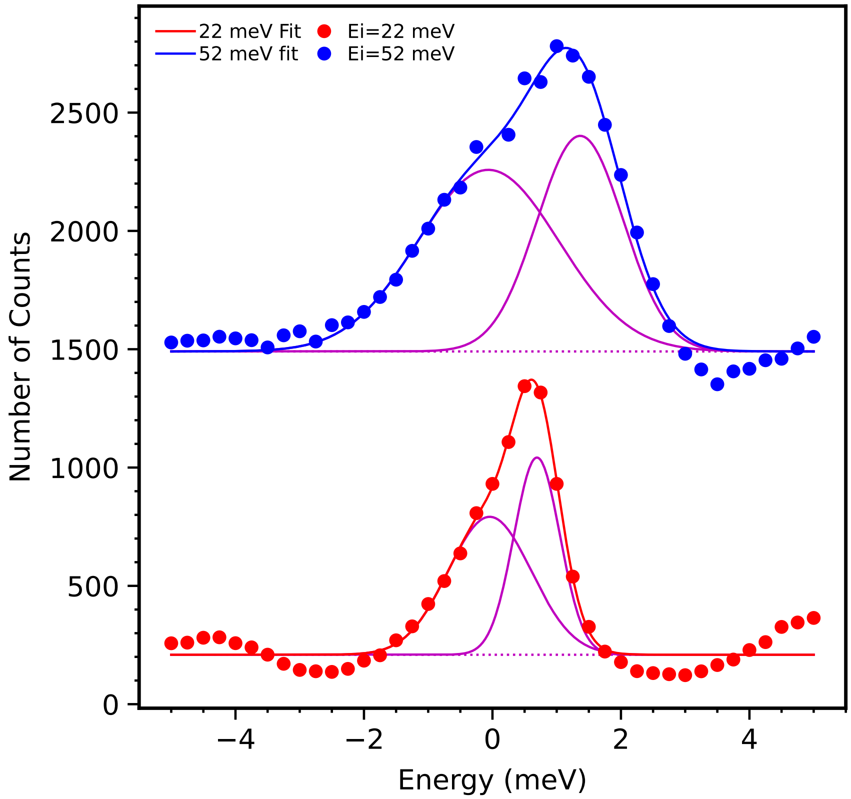


FIG. 3. Results of fitting the experimental resolution. The 52 meV data are offset vertically by 800 counts for clarity. For the 22 meV data, the peaks have widths $w_L^{(22)} = 1.53$ and $w_R^{(22)} = 0.84$ meV from left to right respectively. The ratio of thier heights is $h_L^{(22)}/h_R^{(22)} = 0.70$. The left peak is centered at $c_L^{(22)} = -0.04$ meV and the right at $c_R^{(22)} = 0.69$ meV. For the 52 meV data, the results of the fits are $w_L^{(52)} = 2.59$ and $w_R^{(52)} = 1.58$ meV, $h_L^{(52)}/h_R^{(52)} = 0.84$, and $c_L^{(52)} = -0.06$ and $c_R^{(52)} = 1.37$ meV.

peaks. This is the *elastic* resolution, but we use it for all energy transfers in the GDoS calculations in the main text. The lineshape is asymmetric. We fit it as a sum of two Gaussians. The results are summarized in Fig. 3.

## III. PROJECTED PHONON INTENSITIES

The projected densities of states (PDOS) in the main text are integrated across the full Brillouin zone (BZ). Here, we verify that the optical intensities near the anticrossings in the LA and TA modes are from the rattling atoms. We also explain that the disappearance of

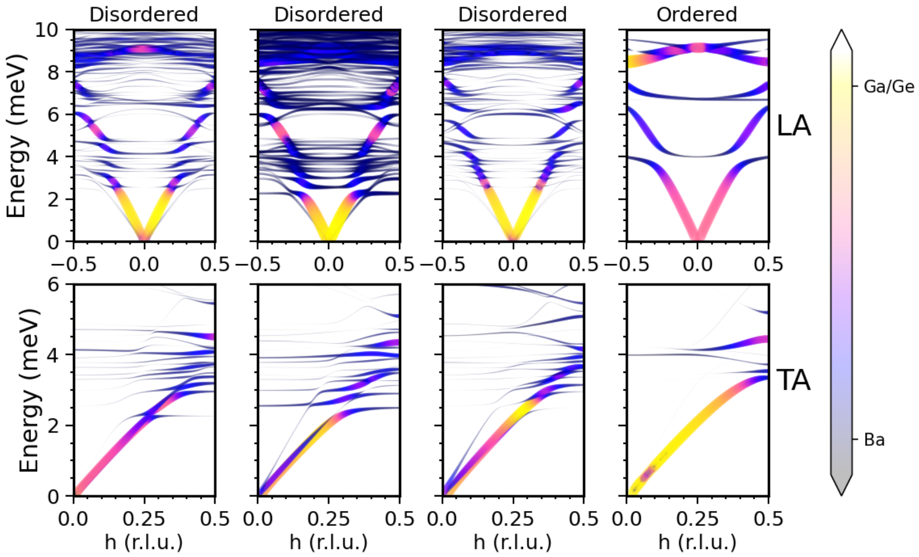


FIG. 4. Inelastic neutron scattering structure factors projected onto the Ba and Ga/Ge atoms. The marker sizes indicate the structure factor (i.e. the intensity) and the color bar indicates which atom(s) contribute the intensity. Small lines are phonon branches with small intensity and thick lines are phonons with large intensity. The first three columns are structure factors calculated from the disordered cell with different permutations of Cartesian axes. The last column is calculated from the ordered cell (permuted axes are identical). The top row shows longitudinal phonons at **Q**=(6+h,0,0) and the bottom row shows the transverse phonons at **Q**=(6,h,0). These and nearby zones were used to fit the dispersions as shown in the main text.

the optical branches at 6 meV in the disordered calculation is not due to vanishing structure factor, but instead is due to loss of degeneracy.

We projected the calculated inelastic neutron scattering intensities onto different atoms by setting the scattering lengths of the rest of the atoms in the unit cell to 0. The results of this procedure are shown in fig. 4 below.

The intensity from the flat branches near 4 and 6 meV in the **Q**=(6±h,0,0) zone comes mainly Ba atoms, while intensity from the flat branches near 4 meV in the $\mathbf{Q}=(6,h,0)$ zone comes mainly from the Ba atoms with some intensity from Ga/Ge atoms near the zone-boundary. In the ordered cell, these branches are multiply degenerate and all contribute some intensity to the spectrum. Their intensities add to appear as a weak but visible flat mode that is present across the whole BZ. Notably, there is no intensity observed in the experiment in the **Q**=(6±h,0,0) zones at this energy except in the vicinity of the LA phonon

peak. Similarly, in the **Q**=(6,h,0) zone in Fig. 4 in the main text, the TA mode appears linear and continuous in the experiment with no visible optic modes nearby.

In the disordered phase calculations, the branches are split due to the broken symmetry. Since the wave vectors **Q** with permuted axes are no longed equivalent, S(**Q**,$\omega$) is averaged over each direction. The averaging over each direction, (and in an experiment, over an ensemble of different disordered unit cells) suppresses and broadens the observed intensity of the flat modes and there is only substantial intensity near the acoustic branches, consistent with experiment. Thus, the flat optical modes present in the ordered calculation that are suppressed in the disordered calculation are mainly due to the Ba rattler atom modes.

## IV. HEURISTIC EXPLANATION OF LOW *AVERAGE* GROUP VELOCITY

The large-gap avoided crossings apparent in the experimental data already flatten the acoustic modes, which reduces the average group velocity. These avoided crossings are due to the presence of the Ba rattler atom and are not from disorder [1]. This flattening would already contribute to lowering the lattice thermal conductivity in $Ba_8Ga_{16}Ge_{30}$. Moreover, our calculations suggest that there may be more avoided crossings present in the material due to the splitting of the rattler modes than are apparent in the experimental INS spectra. There are no splittings visible in the either the experimental or (with reasonably assumed broadening) theoretical INS spectra. Sufficiently "small-gap" avoided crossings can not be resolved by the experiment.

These additional avoided crossings would significantly reduce the average group velocity of the acoustic phonons beyond what is apparent by naively fitting a straight line (SI fig. 5). For sufficiently small gaps and moderate line widths, acoustic branch like intensity composed of numerous avoided crossings between split optical phonons would appear identical to a continuous, linear dispersing acoustic branch (SI figs. 5 a) and d)). The intensity in figure 5 is from a model acoustic phonon with group velocity ∼21 (/ps). The intensity in SI figure 5 d) is from numerous model optical branches with large structure factors only in the vicinity of the acoustic phonon in a). Importantly, the model INS intensity in d) is indistinguishable from a), while the average group velocity in d) (∼3 (/ps)) is 7 times smaller.

Since we cannot observe the splittings in the experimental spectra, it is not clear that the additional small-gap splittings predicted by DFT in the disordered phase are present in the

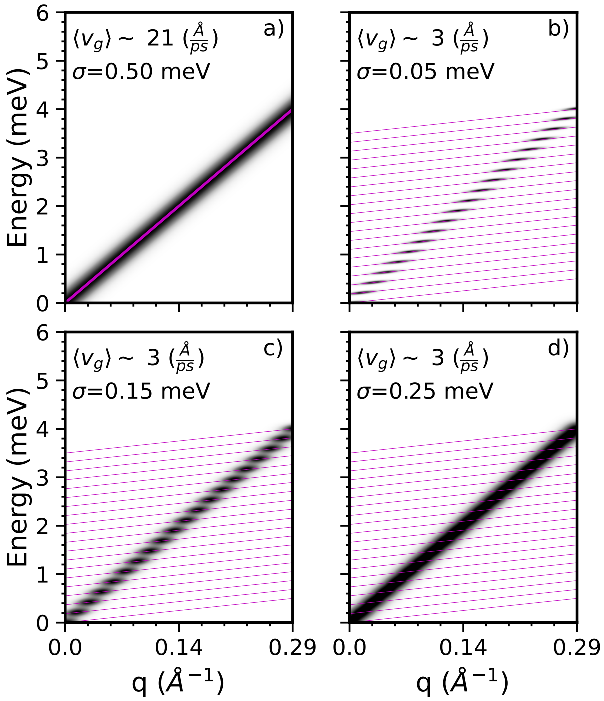


FIG. 5. Heuristic figure indicating how an acoustic phonon with many avoided crossings can appear to be continuously dispersing. a) shows a model acoustic phonon with group velocity $\sim$4 ($/s$), comparable to an acoustic phonon in the main text. b)-d) show closely spaced model optical phonons with intensity only in the region of the acoustic phonon in a). These branches are comparable to the split rattler atom modes in SI fig. 4 and in the main text. The colormaps are structure factors broadened with the FWHMs (indicated in the figures as $\sigma$). With relatively small 0.25 meV broadening in d), the small splittings in c) are already concealed and the intensity is indistinguishable from a continuously dispersing acoustic phonon. However, the average group velocity in d) is 7 times smaller than in a).

experimental spectrum. However, the significantly improved agreement of the disordered phase calculation with experiment over the ordered phase calculation is a strong indication that the splittings are there. Moreover, as explained above, averaging over disordered configurations suppresses and broadens the rattler atom intensity, consistent with the disordered calculation and experiment. Our DFT calculations show that additional splittings due to disorder are present in both the LA and TA phonons along both the [h 0 0] directions in this work and the [h h 0] directions in ref. [1]. If the splittings are present, the severely reduced average group velocity of acoustic bands away from the already flattened large-gap avoided

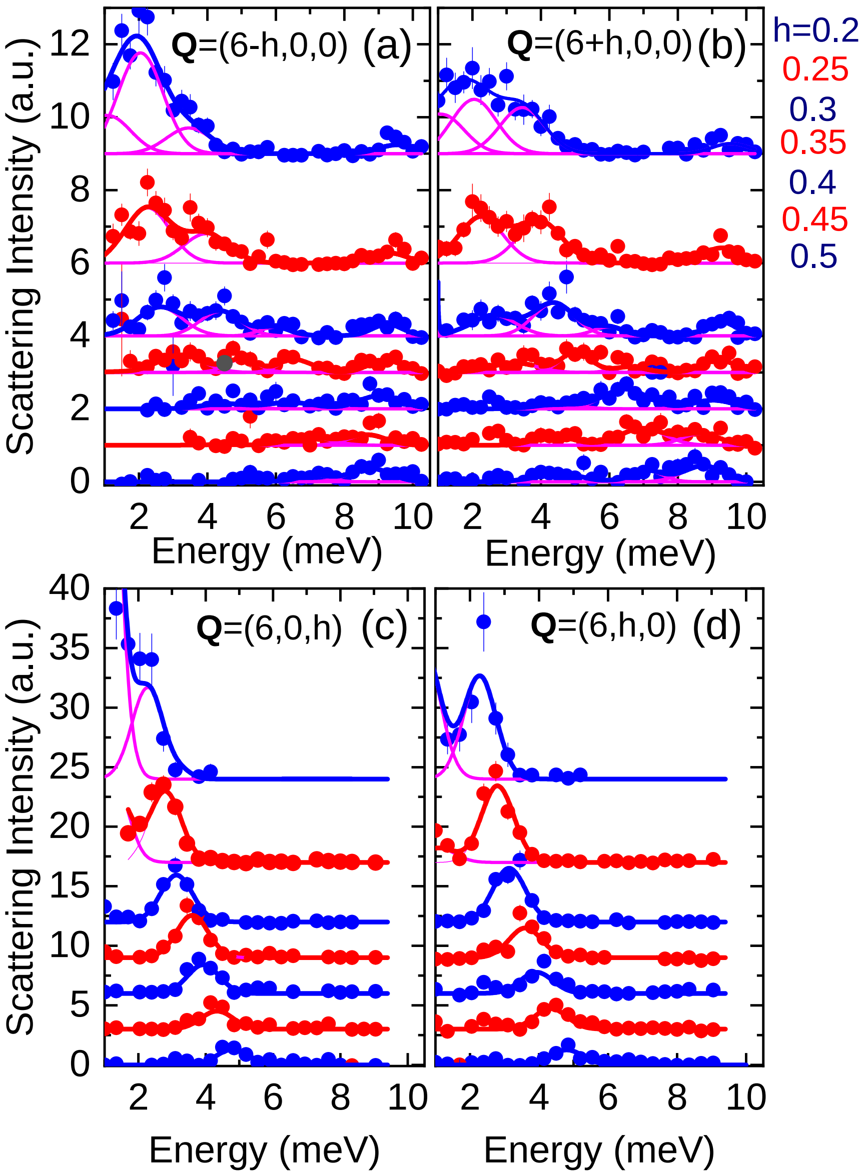


FIG. 6. Constant-q scan of phonons near (6 0 0) along the [h 0 0] and symmetry-equivalent directions of $Ba_8Ga_{16}Ge_{30}$. The data points are raw data after subtracting a constant background. Blue curves are the fit results for h = 0.2, 0.3, 0.4, 0.5 and red are for h = 0.25, 0.35, 0.45. The magenta curves represent the individual phonon peaks obtained after multizone fit.

crossing regions could explain the anomalously low thermal conductivity in $Ba_8Ga_{16}Ge_{30}$.

## V. RESULTS OF MULTIZONE FIT IN PHONON EXPLORER SOFTWARE : CALCULATION OF PHONON ENERGIES

Figure 6 shows background-subtracted phonon spectra along high symmetry directions near strong Q=[6,0,0] Bragg peaks together with results of the multizone fit [3] implemented in Phonon Explorer software [4, 5]. This fit of the phonon spectra in different Brillouin zones constrains peak positions and linewidths to be the same for same reduced wavevectors **q**. Panels (a) and (b) showing phonons at Q=(6-h 0 0) and (6+h 0 0) respectively, select longitudinal branches whereas panels (c) and (d) show data that select transverse branches. Since the data are obtained near one of the strongest Bragg peaks, acoustic phonons should have the strongest intensity whereas the optic modes should be weaker. The TA spectra are dominated by a single peak in figs. 6 (c) and (d), so identifying the TA phonon energies with high accuracy from the multizone fit is straightforward (Fig. 3(b) in the main text). In contrast, the longitudinal phonons in figs. 6 (a) and (b) are mostly broad, because each **q** contains several overlapping peaks whose intensities vary from zone to zone. The LA phonon should always be the strongest. At h = 0.2, it appears at 2 meV whereas the weaker 3.4 meV phonon is LO. At h = 0.25 and 0.3 for both BZs, the two phonons near 2 and 4 meV have LA character as they both have similarly strong intensity. The 6 meV phonon at the same wavevectors is LO as it is less intense. At h=0.35, the intermediate peak at 5 meV is LA as it is more intense than the other two modes at 3 meV and 6.6 meV, especially in the (6+h 0 0) zone. At h=0.4, 0.45, 0.5, the 4 meV phonon is LO whereas the peak near 6.6 meV is LA since it is stronger than the 4 meV peak at **Q**=(6+h 0 0). Note that the LO modes appear whenever there is an avoided crossing with the LA branch below 7 meV for each $h \geq 0.2$. The avoided crossing mixes the eigenvectors of LA and LO branches and repels their corresponding energies. This admixture of LA character makes the LO modes observable near strong Bragg peaks. Our data also contain a pure LO branch near 9.5 meV that does not mix with the LA branch. This experimentally calculated energies are plotted in phonon dispersion shown in fig. 3 in the main text.

---

[1] M. Christensen, A. B. Abrahamsen, N. B. Christensen, F. Juranyi, N. H. Andersen, K. Lefmann, J. Andreasson, C. R. Bahl, and B. B. Iversen, Nature materials **7**, 811 (2008).

[2] Y. Takasu, T. Hasegawa, N. Ogita, M. Udagawa, M. A. Avila, K. Suekuni, I. Ishii, T. Suzuki, and T. Takabatake, Physical Review B **74**, 174303 (2006).

[3] D. Parshall, R. Heid, J. L. Niedziela, T. Wolf, M. B. Stone, D. L. Abernathy, and D. Reznik, Physical Review B **89**, 064310 (2014).

[4] D. Reznik, Phonon-explorer, https://github.com/dmitryr1234/Phonon-Explorer.

[5] D. Reznik and I. Ahmadova, Quantum Beam Science **4**, 41 (2020).
